# Supplementary material for: Hierarchical control strategy for planar bipedal walking robots based on reduced order model
Source: arXiv:2303.12180 source file (2023-02-12)
Supplement: Supplementary file 1 [file Appendix_01.tex]

\chapter{Appendix}
\label{chapter:appendix}

Your appendix should go here.
